# Supplementary material for: Pragmatic factors in image description: the case of negations
Source: arXiv:1606.06164 source file (2016-06-27)
Supplement: Supplementary file 1 [file appendix.tex]

\onecolumn
\appendix
\section*{Appendix A. Example images from the Flickr30K dataset}
Figure \ref{fig:images} provides a sample of the images from the Flickr30K dataset, with their descriptions and categories for those descriptions. These correspond to examples mentioned in the paper.

\begin{figure}[h!]%
\centering
\subfloat[][image 39397486]{\includegraphics[width=0.3\textwidth]{images/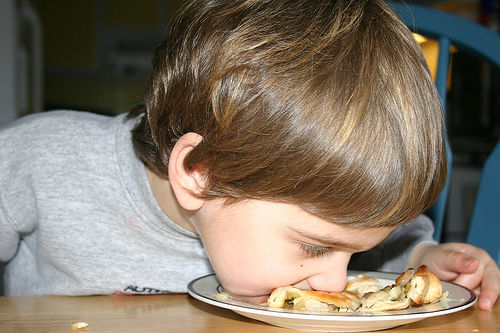}}\quad % Negation of action
\subfloat[][image 2313609814]{\includegraphics[width=0.3\textwidth]{images/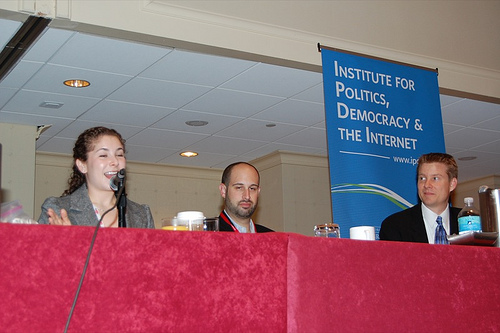}}\quad % attitude
\subfloat[][image 261883591]{\includegraphics[width=0.3\textwidth]{images/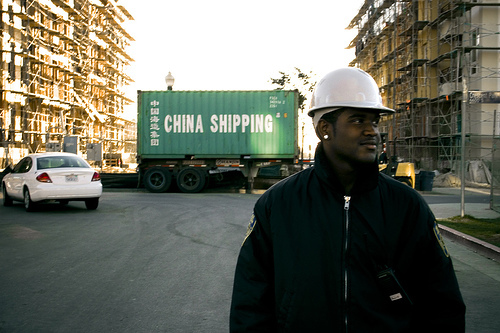}}\\ % Neg of property
\subfloat[][image 13880312]{\includegraphics[width=0.3\textwidth]{images/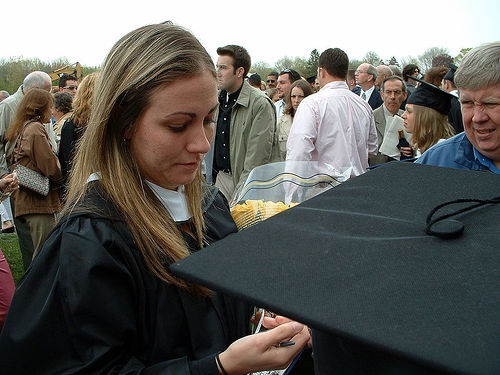}}\quad % Salient absence
\subfloat[][image 4870785283]{\includegraphics[width=0.3\textwidth]{images/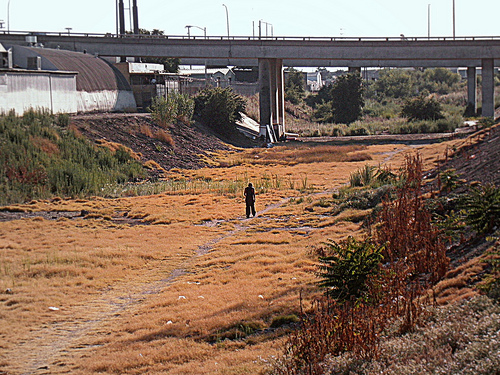}}\quad % Q&I
\subfloat[][image 4895028664]{\includegraphics[width=0.3\textwidth]{images/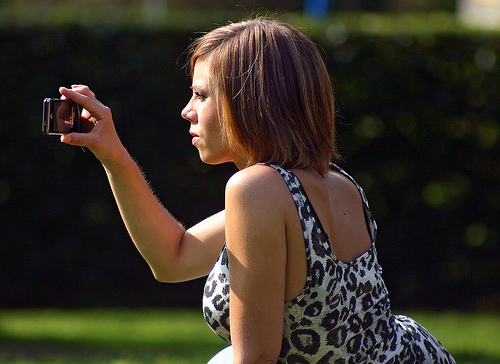}}\\ % outside
\subfloat[][image 263428541]{\includegraphics[width=0.3\textwidth]{images/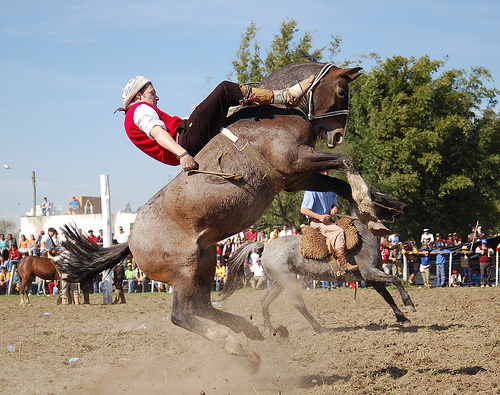}}\quad % future
\subfloat[][image 371522748]{\includegraphics[width=0.3\textwidth]{images/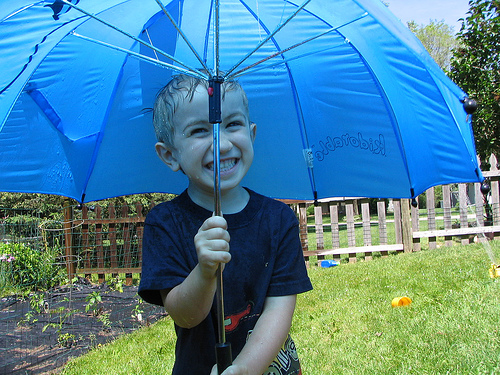}}\quad % other
\subfloat[][image 5954497151]{\includegraphics[width=0.3\textwidth]{images/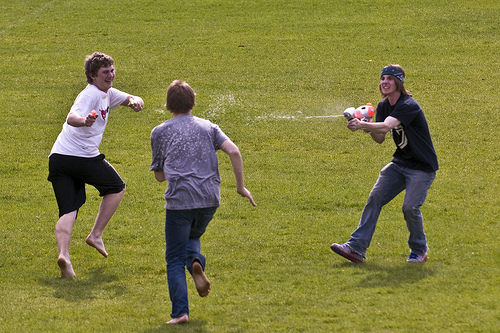}} % contrast
\caption{Images with descriptions containing negations. 
%Categories not shown are \emph{false positive} and \emph{not a description/meta}. 
The categories and descriptions are as follows:\\[5px]
\begin{tabular}{llp{9.8cm}}
\toprule
   & Category & Sentence \\
\midrule
1a & Negation of action/behavior & A kid eating out of a plate \textbf{without} using his hands. \\
1b & Negation of attitude & A man sitting on a panel \textbf{not} enjoying the speech.\\
1c & Negation of property & A man wearing a hard hat stands in front of buildings \textbf{not} yet finished being built. \\
1d & Salient absence & A woman at graduation \textbf{without} a cap on.\\
1e & Quotes \& Idioms & Strolling down path to \textbf{nowhere}. \\
1f & Outside the frame & A woman is taking a picture of something \textbf{not} in the shot with her phone.\\
1g & (Preventing) future events & A man is riding a bucking horse trying to hold on and \textbf{not} get thrown off.\\
1h & Other & The little boy in the blue t-shirt is smiling under the blue umbrella even though it is \textbf{not} raining.\\
1i & Contrast & Three teenagers, two \textbf{without} shoes having a water gun fight with various types of guns trying to spray each other.\\
\bottomrule
\end{tabular}
}%
\label{fig:images}%
\end{figure}
